# Supplementary material for: Evolution of $K$-means solution landscapes with the addition of dataset outliers and a robust clustering comparison measure for their analysis
Source: arXiv:2306.14346 source file (2023-06-25)

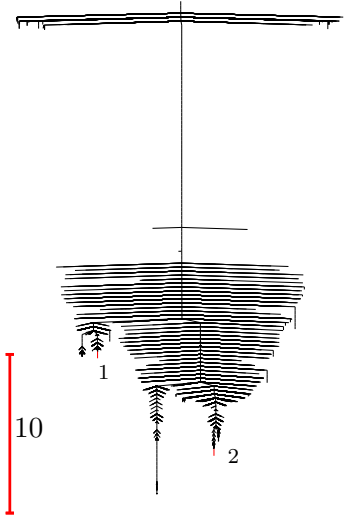

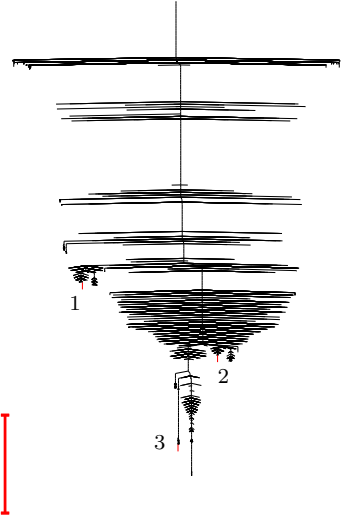

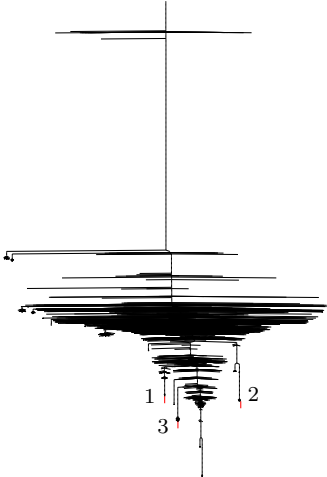

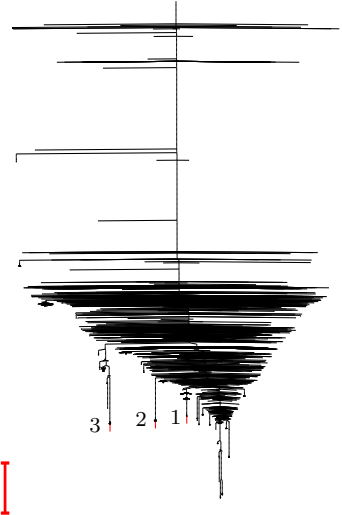

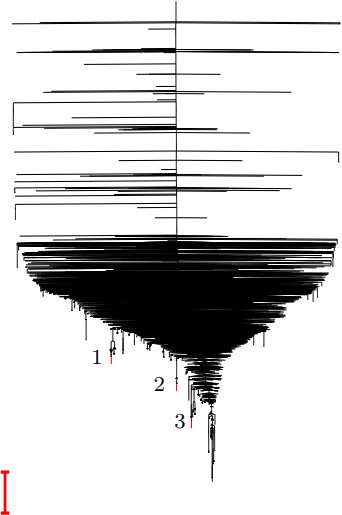

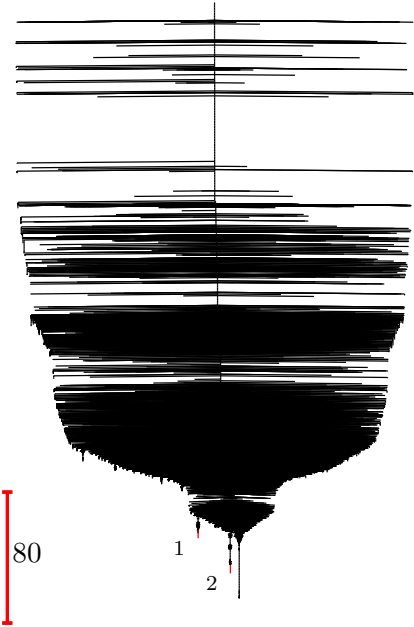

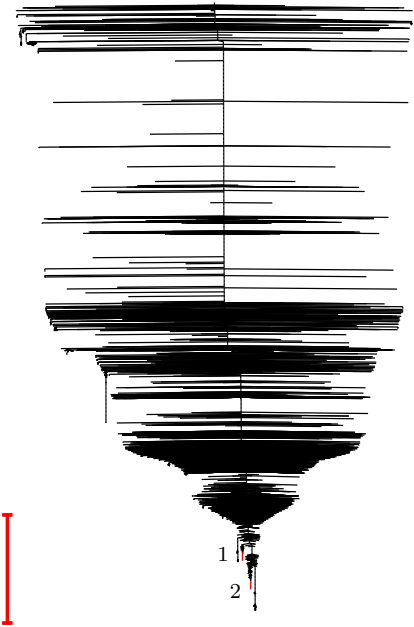

I

2

1

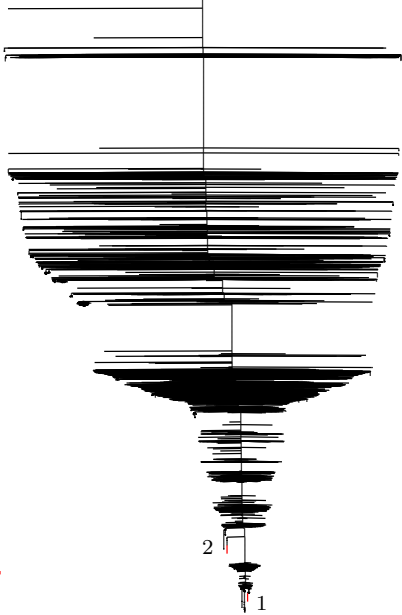



I

1

2

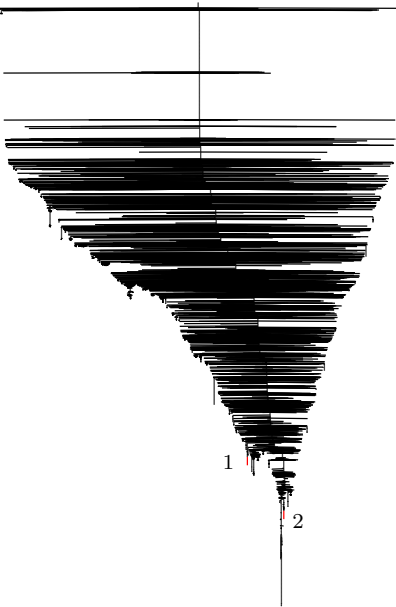

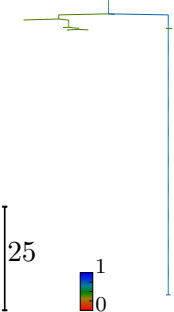

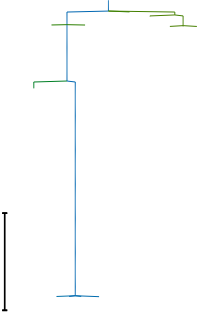

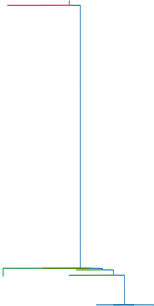

I

I

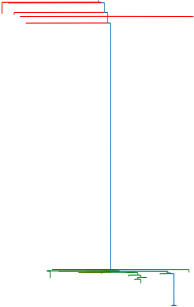

I

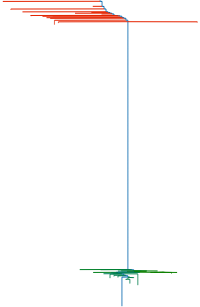

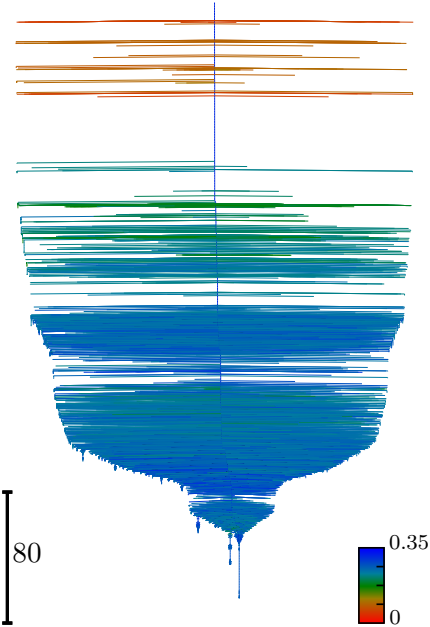

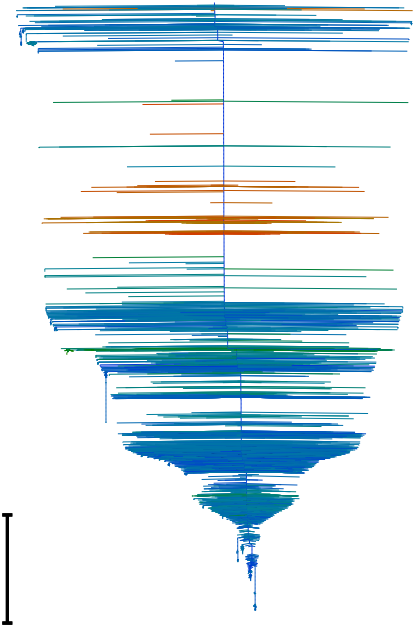



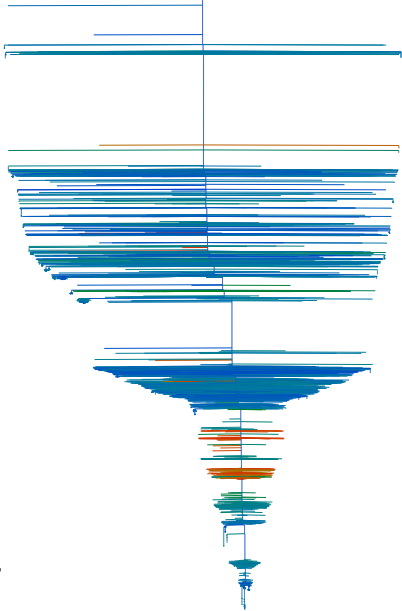

I

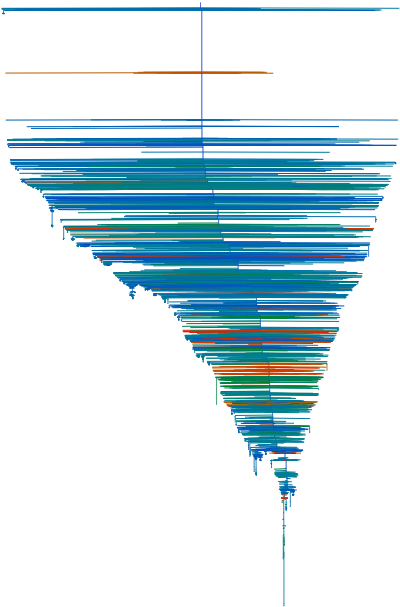

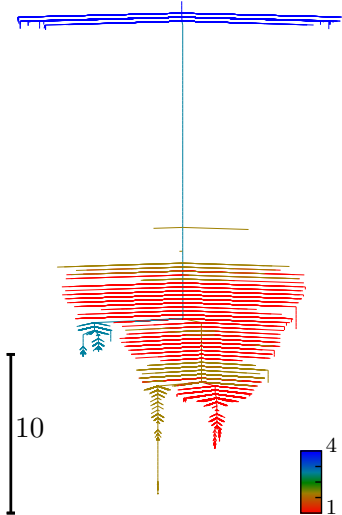

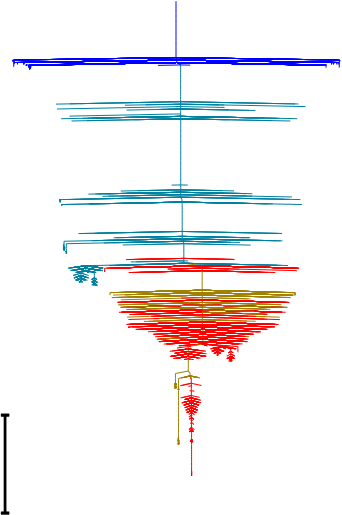

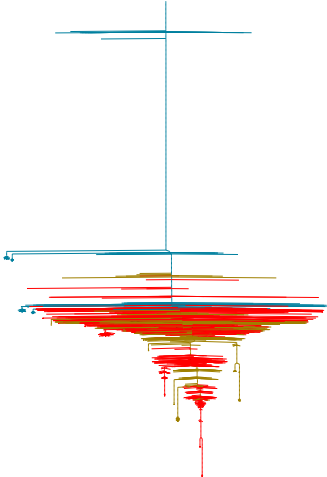

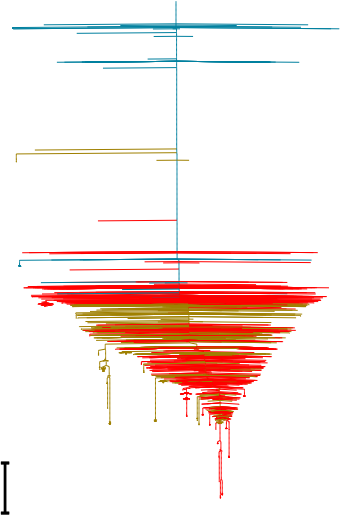

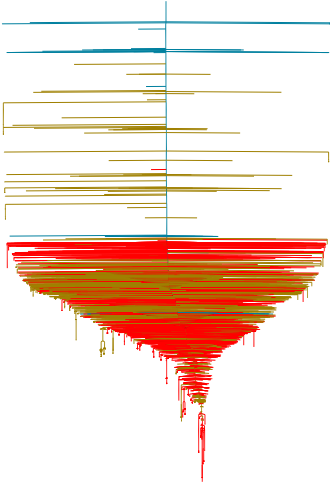

Supplement: Supplementary file 1 [file Outliers_SupportingInformation-pics.pdf]
